# Supplementary material for: Spatio-temporal characterization of nonlinear forcing and response in turbulent channel flow
Source: arXiv:2503.06915 source file (2025-03-10)
Supplement: Supplementary file 1 [file appendix.tex]

\section{The Resolvent Operator}\label{app:resolvent}
Following \citet{mckeon2010}, the primitive form resolvent operator $\mathcal{H}_p(\bm{k},y)$, which maps the forcing $\bm{{f}}$ to the velocity and pressure $[\bm{{u}}, p]^T$ can be written as:
\begin{equation}
	\setlength{\arraycolsep}{0pt}
	
	\mathcal{H}_p(\bm{k},y) = \left(
	-i\omega \left[ 
	\begin{array}{>{\centering\arraybackslash$} p{0.6cm} <{$}>{\centering\arraybackslash$} p{0.6cm} <{$}} 
		\bm{I} & \qquad \\ \qquad & 0 
	\end{array} 
	\right] - \left[ 
	\begin{array}{>{\centering\arraybackslash$} p{0.8cm} <{$}>{\centering\arraybackslash$} p{0.8cm} <{$}} 
		\mathcal{L}_{\bm{k}} & -\nabla_{\bm{k}} \\ \nabla_{\bm{k}}^\mathrm{T} & 0 
	\end{array} 
	\right] \right)^{-1} 
	\begin{bmatrix}
		\bm{I}\\ 0 
	\end{bmatrix},
	\label{eq:H}
\end{equation}
with $\bm{I}$ as the $3\times3$ identity matrix, $\nabla_{\bm{k}}=[ik_x, \frac{d}{dy}, ik_z]^\mathrm{T}$, $\nabla_{\bm{k}}^\mathrm{T}$ the Fourier-transformed gradient and divergence operators, and $\mathcal{L}_{\bm{k}}$ defined as:
\begin{equation}
	\setlength{\arraycolsep}{0pt}
	
	\mathcal{L}_{\bm{k}} =
	\left[ \begin{array}{ccc}
		-ik_x\overline{U} + \frac{\Delta_{\bm{k}}}{\Rey} & -\frac{ d \overline{U}}{d y}& 0 \\
		0 & -ik_x\overline{U} + \frac{\Delta_{\bm{k}}}{\Rey} & 0 \\
		0 & 0 & -ik_x\overline{U} + \frac{\Delta_{\bm{k}}}{\Rey} \\
	\end{array} \right],
	\label{eq:lk}
\end{equation}
where $\Delta_{\bm{k}} = \frac{d^2}{dy^2} - k_x^2 - k_z^2$ is the Fourier-transformed Laplacian. Note that the primitive form resolvent operator $\mathcal{H}_p(\bm{k},y)$ defined in equation~\eqref{eq:H} is a $4\times 3$ operator, mapping the three forcing components to the three velocity components plus the pressure. Since pressure is not studied in this work, the last row of $\mathcal{H}_p$ can be removed to obtain the $3\times 3$ operator, $\mathcal{H}(\bm{k},y)$, mapping the three forcing components to the three velocity components without giving the pressure. Alternatively, similar to~\citet{moarref2013}, the wall normal velocity $v$ and wall normal vorticity $\eta =  i k_z u - i k_x w$ can be used to eliminate the pressure and derive $\mathcal{H}(\bm{k},y)$ utilizing the Orr-Sommerfeld and Squire operators.

\section{Temporal Filtering to Remove Temporal Aliasing in the Forcing} \label{app:lpf}
A low pass filter (LPF) with cutoff frequency $f_c$ is inserted into the DNS before sampling the velocities, and only frequencies in the range of $\bracket{-f_R, f_R}$ from the temporal Fourier transform of the sampled data are retained. The resolved frequency range is required to be smaller than the cutoff frequencies $f_R \leq f_c$, and additional requirements come from consideration of the quadratic forcing terms. Assuming a LPF with infinite roll-off at $f_c$, the non-linear forcing will have its highest frequency at $2f_c$ aliasing to $2f_c - 2f_{s,NQ}$, which should remain outside of the resolved zone:
\begin{equation}
	2f_c - 2f_{s,NQ} \leq - f_R, 
\end{equation}
where $f_{s,NQ} = \frac{1}{2 \Delta t_s}$ is the sampling Nyquist frequency. When setting $f_R = f_c$, the 2/3 dealiasing result of $f_R \leq \frac{2}{3}f_{s,NQ}$ is obtained, similar to that used in the spatial dimensions. However, to account for the LPF having a finite roll-off at the cutoff frequency, some buffer is introduced by selecting:
\begin{equation}
	f_R = \frac{1}{2} f_{s,NQ}.
\end{equation}
This filter design is guaranteed to remove all aliasing in the forcing under the worst-case scenario. Practically, very little energy content is present for the forcing at the very high frequencies, and the filter criterion could be relaxed slightly to retain more of the higher frequencies, with the trade-off of allowing small amounts of energy at the high frequencies to cause aliasing. 

Additionally, no phase distortion of the filtered signal is desired, requiring a linear phase filter, where the filter phase response is a linear function of frequencies. This results in a filtered signal with all frequencies having the same constant time delay compared to the unfiltered signal, or in other words, no phase distortion (see appendix~\ref{appendix:lpf}). An order 2000 filter is designed using MATLAB fircls1 function \citep{MATLAB}, with the maximum amplitude deviation set to $10^{-4}$ for the pass band $[0, f_R]$, and $10^{-3}$ for the stop band. The resulting filter amplitude and phase are plotted in Figure~\ref{fig:filter}, which shows the resolved frequency range with very little amplitude deviation from 1 and a perfectly linear phase response.
\begin{figure}
	\centering
	\includegraphics[width=379pt]{{./Figures/Chapter4/FilterDesign}.eps}
	\caption{(\textit{a}) Amplitude and (\textit{b}) phase for the order 2000 linear-phase low pass filter. The vertical lines correspond to  $f_R = \tfrac{1}{2}f_{s,NQ}$, the resolved frequency range, and $\tfrac{2}{3}f_{s,NQ}$, the largest frequency that does not cause aliasing.}
	\label{fig:filter}
\end{figure}

To demonstrate the necessity and effect of the filter, two short DNS runs are conducted with the same parameters as the main computation. The first run does not include the LPF, while the second one includes the LPF as described above. The two runs are initialized using the same initial conditions with the time delay induced by the LPF properly corrected, ensuring the two runs are properly aligned in time. The power spectrum of the wall-normal velocity forcing $f_v$ is computed for both runs and compared in Figure~\ref{fig:fv} at $y = 0.91$ ($y^+ = 500$). $f_v$ is the forcing utilized in the velocity-vorticity resolvent formulation, defined as:
\begin{equation}
	\begin{bmatrix}
		f_v\\ f_{\omega_y}
	\end{bmatrix} = 
	\begin{bmatrix}
		-ik_x \frac{d}{dy} & -k^2 & -ik_z \frac{d}{dy}\\
		i k_z & 0 & - i k_x
	\end{bmatrix}
	\bm{f}(\bm{k},y).
\end{equation}
This is the solenoidal part of the forcing, which excludes the irrotational part that is not responsible for driving the velocities (see the Helmholtz decomposition discussed in \citet{Rosenberg_McKeon_2019_efficient}, and \citet{Morra_Nogueira_Cavalieri_Henningson_2021}). 

In Figure~\ref{fig:fv}, the black dash lines denote the critical layer, where the wavespeed $c = \omega/k_x$ is equal to the local spatio-temporal means velocity $c = \overline{U}(y)$~\citep{mckeon2010}. The frequencies beyond the sampling Nyquist frequency are aliased to the resolved frequency range, which manifests as the ``S'' shaped part of the dashed lines in Figures~\ref{fig:fv}, due to the log scaled axes. The energy in the forcing can be seen to concentrate around the critical layer consistent with previous studies~\citep{Rosenberg_2018}. Starting from $k_x\approx40$, significant energy content can be observed near the aliased ``S'' shaped part of the dashed lines in the unfiltered results presented in the first column. This aliased energy content corrupts the results starting from $k_x\approx40$, showing the necessity of the LPF in the DNS for studying the non-linear forcing. From the power spectra of the filtered run presented in the second column of Figure~\ref{fig:fv}, and the difference between the filtered and unfiltered results presented in the third column, it can be observed that the aliased energy in the forcing is completely removed by the introduction of the LPF, while the non-aliased energy is correctly preserved.
\begin{figure}
	\centering
	\includegraphics[width=368pt]{{./Figures/Chapter4/fv_yp500}.eps}
	\caption{The wall normal velocity forcing $f_{v}$ power spectra in $k_x-\omega$ space at $y = 0.91$ ($y^+ = 500$) for (\textit{a, d}) the unfiltered DNS, and (\textit{b, e}) the filtered DNS. The third column (\textit{c, f}) is the difference between the unfiltered and filtered spectra. The top row (\textit{a-c}) is for positive $\omega$ and the bottom row (\textit{d-f}) for negative $\omega$. The black dashed line in all six subplots denote the critical layer $c = \omega/ k_x = \overline{U}(y=0.91)$ with the $\omega$ frequencies beyond the sampling Nyquist frequency aliasing into the resolved frequency range, manifesting as the ``S'' shaped part of the dashed lines. }
	\label{fig:fv}
\end{figure}

It is also observed that the aliased energy predominately resides in regions with $k_x \geq 40$ for $y^+ = 500$ as shown in Figures~\ref{fig:fv}. Therefore, removing all $k_x$ wavenumbers above a critical value $k_{x,c}$ could potentially be utilized as an alternative method to inserting a LPF into the DNS code. This critical streamwise wavenumber $k_{x,c}$ differs for each wall-normal location, and can be best estimated using the critical layer location: $k_{x,c}(y) = \omega_{s,NQ} /\overline{U}(y)$, where $\omega_{s,NQ}$ is the sampling Nyquist frequency. However, this method will not remove the aliased energy as cleanly as the LPF, and does not guarantee the complete removal of all aliased energy. In cases where rerunning the simulation with a LPF in the code is not feasible, this might serve as an alternative method.

\section{Derivation of the Spectral Turbulence Kinetic Energy (TKE) Equation} \label{appendix:stke}
In section~\ref{sec2:tke}, we define the spectral turbulence kinetic energy (TKE) as $e(\bm{k},y) = \abs{u(\bm{k},y)}^2 + \abs{v(\bm{k},y)}^2 + \abs{w(\bm{k},y)}^2$, which is the energy of a Fourier modes at given $\bm{k}$. Due to the Hermitian symmetry of the Fourier modes, we have $e(\bm{k},y) = e(-\bm{k},y)$. Starting with the Fourier transformed NSE:
\begin{alignat}{5}
	&\bracket{-i\omega + i k_x \overline{U}(y) + \frac{k^2}{\Rey} - \frac{1}{\Rey} \frac{d^2}{dy^2} } u(\bm{k},y)&&+\overline{U}'(y) v(\bm{k},y)&&+ik_x        &&p(\bm{k},y) &&= f_x(\bm{k},y),\\[0.5em]
	&\bracket{-i\omega + i k_x \overline{U}(y) + \frac{k^2}{\Rey} - \frac{1}{\Rey} \frac{d^2}{dy^2} } v(\bm{k},y)&&                             &&+\frac{d}{dy}&&p(\bm{k},y) &&= f_y(\bm{k},y),\\[0.5em]
	&\bracket{-i\omega + i k_x \overline{U}(y) + \frac{k^2}{\Rey} - \frac{1}{\Rey} \frac{d^2}{dy^2} } w(\bm{k},y)&&                             &&+ik_z        &&p(\bm{k},y) &&= f_z(\bm{k},y),
\end{alignat}
with $\overline{U}'(y) = \frac{d \overline{U}(y)}{d y}$. Multiply the three equations with $u^*(\bm{k},y)$, $v^*(\bm{k},y)$, $w^*(\bm{k},y)$, take the sum, and utilize continuity to obtain:
\begin{align}
	&\bracket{-i\omega + i k_x \overline{U}(y) + \frac{k^2}{\Rey} } e(\bm{k},y) +  u^*(\bm{k},y) v(\bm{k},y) \overline{U}'(y) + \frac{d}{dy} \bracket{ v^*(\bm{k},y) p(\bm{k},y)} \nonumber\\[0.5em]
	&- \frac{1}{\Rey}\bracket{ u_i^*(\bm{k},y) \frac{d^2}{dy^2} u_i(\bm{k},y) } = u_i^*(\bm{k},y) f_i(\bm{k},y),
\end{align}
where the summation notation is used with the subscript $i$. We then add it with the equation for $e(-\bm{k},y)$, and utilized $e(\bm{k},y) = e(-\bm{k},y)$ and the symmetry of Fourier modes $u^*(\bm{k},y) = u(-\bm{k},y)$ to obtain:
\begin{align}
	& \underbrace{
		\real{ u^*(\bm{k},y) v(\bm{k},y) \overline{U}'(y) } \vphantom{\frac{d^2}{dy^2}} 
	}_{\text{Production}} 
	+ \underbrace{ 
		\frac{k^2 }{\Rey} e(\bm{k},y) + \frac{1}{\Rey} \frac{d}{dy}u_i^*(\bm{k},y) \frac{d}{dy} u_i(\bm{k},y)
	}_{\text{Viscous Dissipation}} \nonumber\\[0.5em]
	+& \underbrace{
		\real{\frac{d}{dy} \bracket{ v^*(\bm{k},y) p(\bm{k},y)}}
	}_{\text{Pressure Transport}}
	- \underbrace{
		\frac{1}{2} \frac{1}{\Rey} \frac{d^2}{dy^2} e(\bm{k},y) \vphantom{\real{\frac{d}{dy}}} 
	}_{\text{Viscous Transport}} 
	= \underbrace{
		\real{ u_i^*(\bm{k},y) f_i(\bm{k},y) \vphantom{\frac{d}{dy}} }   
	}_{\text{Turbulent Transport}},
\end{align}
where $\real{\cdot}$ indicates the real part. This resembles the form in \citet{Cho_Hwang_Choi_2018}, which is written for the modes Fourier transformed in $z$ only, while we provide the results for the modes Fourier transformed in $x, z, t$.

\section{Importance of Linear Phase Response for Temporal Filtering} \label{appendix:lpf}
In this section, we will show that phase distortion in the pass band can be avoided with a linear phase low pass filter. Since the stop band frequencies have significantly lower amplitude response, it is sufficient to limit the analysis to only the pass band of the filter, with a transfer function $A(\omega) e ^{i\phi(\omega)}$, where $A(\omega)$ is the amplitude, and $\phi(\omega) = - k \omega$ is the linear phase response of the filter. 

Denote a pre-filtered signal containing frequencies only in the pass band as $q(t)$, with Fourier coefficient $\hat{q}(\omega)$ and the filtered signal $q_f(t)$ and $\hat{q}_f(\omega)$, the filtered signal is related to the unfiltered by the filter transfer function:
\begin{equation}
	\hat{q}_f(\omega) = A(\omega) \hat{q}(\omega) e^{i\phi(\omega)} = A(\omega) \hat{q}(\omega) e^{- i k \omega}.
\end{equation}
Utilizing the approximation of $A(\omega) \approx 1$ in the filter pass band and the Fourier transform pair, we obtain:
\begin{equation}
	q_f(t) = \int \hat{q}_f(\omega) e^{i\omega t} d\omega \approx \int \hat{q}(\omega) e^{i\omega t - i k \omega} d\omega = q(t-k),
\end{equation}
which shows that the filtered signal is a time delayed copy of the original signal with no phase distortion in the pass band. This constant time delay can be easily corrected in post-processing, and the next section shows that the time delay does not affect the computation of the interaction coefficients. More rigorous analyses of linear-phase filters can be found in digital filter textbooks such as \cite{Parks_Burrus_1987}.

\section{Validity of the Application of the Welch Method} \label{appendix:welch}
In this section, we will (non-rigorously) show that the Welch method can be correctly applied to the computation of $P(\bm{k}_1,\bm{k}_2)$ and $R(\bm{k}_1,\bm{k}_2)$. For simplicity, we will neglect all spatial coordinates as those do not affect the temporal Fourier analysis, and redefine $P$ and $R$ for this analysis as:
\begin{eqnarray}
	P(\omega_1, \omega_2) &=& \hat{f}^*(\omega_1 + \omega_2) \hat{u}_1(\omega_1) \hat{u}_2(\omega_2), \\
	R(\omega_1, \omega_2) &=& \hat{u}_1^*(\omega_1 + \omega_2) \mathcal{H}(\omega_1 + \omega_2)\hat{u}_1(\omega_1) \hat{u}_2(\omega_2),
\end{eqnarray}
where $\hat{u}_1(\omega)$ is the Fourier coefficient of $u_1(t)$, a proxy for the velocity, $\hat{u}_2(\omega)$ is the Fourier coefficient of $u_2(t)$, a proxy for the velocity gradient, and $\hat{f}(\omega)$ is the Fourier coefficient of $f(t) = u_1(t) u_2(t)$.

The three signals are then shifted in time by a constant $\Delta t$, resulting in their Fourier coefficients shifted in phase:
\begin{equation}
	u_1'(t) = u_1(t + \Delta t) \implies \hat{u}'_1(\omega) = \hat{u}_1(\omega) e^{i \omega \Delta t},
\end{equation}
with $u_2$ and $f$ following the same relation. $P'(\omega_1, \omega_2)$ can therefore be defined for the time shifted signals:
\begin{eqnarray}
	P'(\omega_1, \omega_2) &=& \hat{f}'^*(\omega_1 + \omega_2) \hat{u}'_1(\omega_1) \hat{u}'_2(\omega_2) \nonumber\\
	&=& \bracket{\hat{f}(\omega_1 + \omega_2) e^{i(\omega_1 + \omega_2) \Delta t}}^* \bracket{\hat{u}_1(\omega_1)  e^{i \omega_1 \Delta t}} \bracket{\hat{u}_2(\omega_2)  e^{i \omega_2 \Delta t}} \nonumber\\
	&=&  P(\omega_1, \omega_2)
\end{eqnarray}
which shows that $P(\omega_1, \omega_2)$ is invariant with respect to any time shifts of the signals. With the resolvent operator $\mathcal{H}(\omega)$ also invariant with respect to time shifts, a similar analysis can be applied to $R(\omega_1, \omega_2)$ as well, reaching the same conclusion.

Since the two coefficients are invariant with respect to time shifts, the full time series can be segmented, the coefficients computed for each segment, before taking the average across multiple segments for improved convergence. More rigorously, we are assuming wide-sense stationarity extended to the third order statistics, where the triple correlation depends only on the time differences, similar to the auto-correlation in second order statistics.
